# Supplementary material for: Continual Segment: Towards a Single, Unified and Accessible Continual Segmentation Model of 143 Whole-body Organs in CT Scans
Source: arXiv:2302.00162 source file (2023-09-03)
Supplement: Supplementary file 1 [file appendix.tex]

% CVPR 2023 Paper Template
% based on the CVPR template provided by Ming-Ming Cheng (https://github.com/MCG-NKU/CVPR_Template)
% modified and extended by Stefan Roth (stefan.roth@NOSPAMtu-darmstadt.de)

\documentclass[10pt,twocolumn,letterpaper]{article}

%%%%%%%%% PAPER TYPE  - PLEASE UPDATE FOR FINAL VERSION
% \usepackage[review]{cvpr}      % To produce the REVIEW version
%\usepackage{cvpr}              % To produce the CAMERA-READY version
\usepackage[pagenumbers]{cvpr} % To force page numbers, e.g. for an arXiv version
\input{math_commands.tex}

% Include other packages here, before hyperref.

\usepackage{graphicx}
\usepackage{amsmath}
\usepackage{amssymb}
\usepackage{booktabs}
\usepackage{acro}
\usepackage{amsfonts}
\usepackage{acro}
\usepackage{algorithm2e}
\usepackage{multirow}
\usepackage{booktabs}
\usepackage[table,xcdraw]{xcolor}

\usepackage{xr}

% It is strongly recommended to use hyperref, especially for the review version.
% hyperref with option pagebackref eases the reviewers' job.
% Please disable hyperref *only* if you encounter grave issues, e.g. with the
% file validation for the camera-ready version.
%
% If you comment hyperref and then uncomment it, you should delete
% ReviewTempalte.aux before re-running LaTeX.
% (Or just hit 'q' on the first LaTeX run, let it finish, and you
%  should be clear).
\usepackage[pagebackref,breaklinks,colorlinks]{hyperref}

% Support for easy cross-referencing
\usepackage[capitalize]{cleveref}
\crefname{section}{Sec.}{Secs.}
\Crefname{section}{Section}{Sections}
\Crefname{table}{Table}{Tables}
\crefname{table}{Tab.}{Tabs.}

% refer to separate appendix.tex
\externaldocument[M-]{PaperForReviewCVPR2023_v1}

% \usepackage{xr}
% \makeatletter
% \newcommand*{\addFileDependency}[1]{% argument=file name and extension
%   \typeout{(#1)}
%   \@addtofilelist{#1}
%   \IfFileExists{#1}{}{\typeout{No file #1.}}
% }
% \makeatother

% \newcommand*{\myexternaldocument}[1]{%
%     \externaldocument{#1}%
%     \addFileDependency{#1.tex}%
%     \addFileDependency{#1.aux}%
% }
% \myexternaldocument{test}

\SetKwInput{KwData}{Input}
\SetKwInput{KwResult}{Output}

% \DeclareAcronym{RTCT}{
% short=RTCT,
% long=radiotherapy computed tomography
% }

% \DeclareAcronym{p3d}{
% short=P3D,
% long=Pseudo-3D
% }

% \DeclareAcronym{nas}{
% short=NAS,
% long=neural architecture search
% }

% \DeclareAcronym{dsc}{
% short=DSC,
% long=Dice score
% }

% \DeclareAcronym{hd}{
% short=HD,
% long=Hausdorff distance
% }

% \DeclareAcronym{hd95}{
% short=HD95,
% long=Hausdorff distance 95\%
% }

% \DeclareAcronym{asd}{
% short=ASD,
% long=average surface distance
% }

% \DeclareAcronym{ge}{
% short=GE,
% long=General Encoder,
% foreign-plural={}
% }

% \DeclareAcronym{gs}{
% short=ContinualSeg,
% long=Continual Segment,
% foreign-plural={}
% }

% \DeclareAcronym{fov}{
% short=FOV,
% long=field of view,
% foreign-plural={}
% }

% \DeclareAcronym{fbkg}{
% short=FBkg,
% long=fake background,
% foreign-plural={}
% }

\DeclareAcronym{kd}{
short=KD,
long=knowledge distillation,
foreign-plural={}
}

%%%%%%%%% PAPER ID  - PLEASE UPDATE
 % *** Enter the CVPR Paper ID here

\begin{document}

\title{Supplementary Material: Towards a Single, Unified and Accessible Continual Segmentation Model of 143 Whole-body Organs in CT Scans}
% Continual Segment: Towards a Single, Unified and Accessible Continual Segmentation Model of 143 Whole-body Organs in CT Scans

% \author{First Author\\
% Institution1\\
% Institution1 address\\
% {\tt\small firstauthor@i1.org}
% % For a paper whose authors are all at the same institution,
% % omit the following lines up until the closing ``}''.
% % Additional authors and addresses can be added with ``\and'',
% % just like the second author.
% % To save space, use either the email address or home page, not both
% \and
% Second Author\\
% Institution2\\
% First line of institution2 address\\
% {\tt\small secondauthor@i2.org}
% }

\maketitle

\appendix
\counterwithin{figure}{section}
\counterwithin{table}{section}

\tableofcontents

% ==================== Extended related work ====================
% \section{Extended Related Work}
% \label{supp:related}
% ==================== Dataset statistics ====================
\section{Dataset Details}
\label{supp:dataset}
\input{app_dataset.tex}
% train:test, organ list, body parts
% ==================== Implementation Details ====================
\section{Implementation Details}
\label{supp:implement}
\input{app_implement.tex}
% nnUNet hyperparams
% NAS / Pruning details - final network structure of each decoder
% Merging - body parts partition of each dataset
% ==================== Ablation Studies and Result Analysis ====================
%Additional Ablation Studies and Result Analysis
\section{Additional Ablation Results and Analysis}
\label{supp:ablation}
\input{app_ablation.tex}
% More result analysis of each comparison methods in main paper (Tab 1-2; Fig 4)
% Detailed table (numeric values) of Fig 4
% More figures and tables (forgetting rate, HD95/ASD of Fig.4?)
% Pretrained encoder on different dataset (w. or w/o fake bkg) --> 1-step CIS
% More ...
% ==================== Ablation Studies and Result Analysis ====================
\section{Detailed Results of Individual Organs}
\label{supp:organ}
\input{app_organ.tex}
% Detailed organ-wise results of each upperbound
% Ours: detailed results of each organ in each dataset (How to demonstrate TotalSeg results?)
% All methods: box-plots of all organs (mean/std)? 
% More ...
% ==================== Reimplementation of Comparison Methods ====================
\section{Reimplementation of Comparison Methods}
\label{supp:impl_comp}
\input{app_impl_comp.tex}
% MiB, ILT, PLOP, LISMO
% \clearpage

% % ==================== More Segmentation Samples ====================
% \section{Additional Figures}
% \label{supp:figure}
% more segmentation samples
% merging results - naive ensamble vs. our method (FPR using body part mask)

%%%%%%%%% REFERENCES
{\small
\bibliographystyle{ieee_fullname}
\bibliography{egbib, ref_ciss}
}

\end{document}
